# Supplementary material for: MultiMorph: On-demand Atlas Construction
Source: arXiv:2504.00247 source file (2025-03-31)
Supplement: Supplementary file 1 [file appendix.tex]

\section{Appendix}
\subsection{Hyperparameter Evaluation}
\label{app:hyperparam}

\begin{figure}[!h]
    \centering
    \includegraphics[width=\linewidth]{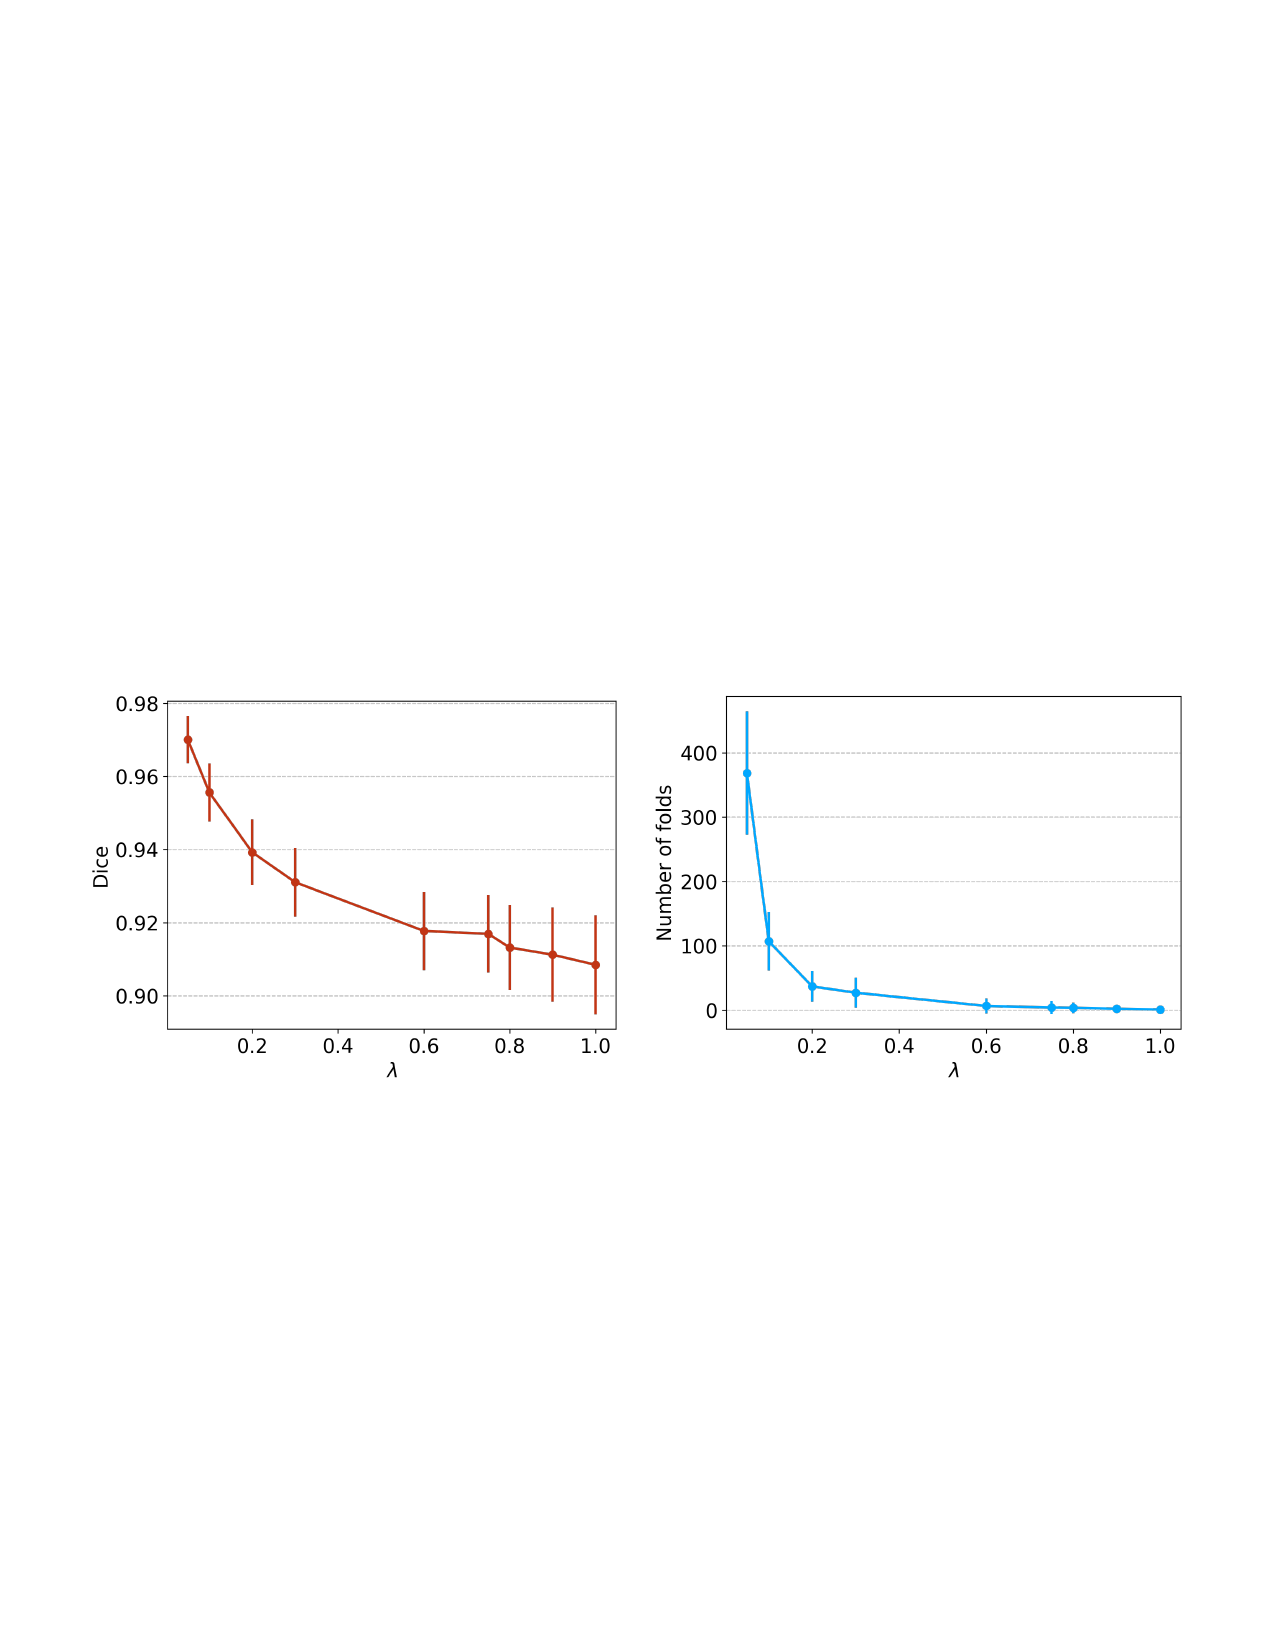}
    \caption{Hyperparameter sweep for field regularization parameter $\lambda$ for the OASIS1 validation set.}
    \label{fig:hyperparam}
\end{figure}
