# Supplementary material for: MultiMorph: On-demand Atlas Construction
Source: arXiv:2504.00247 source file (2025-03-31)
Supplement: Supplementary file 2 [file supplement.tex]

\appendix
\section{Corrected Aladdin Results}
test
